# Supplementary material for: DiffusionNAG: Predictor-guided Neural Architecture Generation with Diffusion Models
Source: arXiv:2305.16943 source file (2024-03-24)
Supplement: Supplementary file 1 [file tbl_suppl_guidance.tex]

\begin{table}[t!]
\caption{\small \textbf{Validity Results - Coarse Grid Search} }
\vspace{-0.1in}
\tiny
\begin{center}
\resizebox{0.5\linewidth}{!}{
\begin{tabular}{cccc}
\toprule
Guidance Strength  & $10^6$     & $10^5$ & \textbf{$10^4$} \\
                           
\midrule
\midrule
Validity                 & 0.0               & 0.0 & \textbf{100.0}   \\
\bottomrule
\end{tabular}
} 	
\end{center}
\label{tbl:suppl_guidance}
\vspace{-0.15in}
\end{table}
