# Supplementary material for: DiffusionNAG: Predictor-guided Neural Architecture Generation with Diffusion Models
Source: arXiv:2305.16943 source file (2024-03-24)
Supplement: Supplementary file 2 [file tbl_suppl_guidance_abl.tex]

\begin{table}[t!]
\caption{\small \textbf{Ablation Study - Guidance Strength} Distribution of generated neural architectures across various sampling strategies. All methods generated neural architectures within the same sampling time. }
\vspace{-0.1in}
\tiny
\begin{center}
\resizebox{1.0\linewidth}{!}{
% {\color{blue}\begin{tabular}{cccc}
% \toprule
% Stats.  & Fixed at a large value    & Balanced exploitation-exploration  
% (Ours) & Fixed at a small value  \\
                           
% \midrule
% \midrule
% Max Accuracy (\%)                                   & 94.3633 & \textbf{94.3733} & \textbf{94.3733} \\ 
% Mean Accuracy (\%)                                  & 93.4658 & 93.1881 & 93.0640 \\ 
% Min Accuracy (\%)                                   & 90.6450 & 89.9367 & 88.1767 \\ 
% Standard Deviation (\%)                             & 1.0334  & 1.2118  & 1.4169  \\ 
% Avg. Acc. of Top-5 (\%) & 93.9880 & \textbf{94.2477} & 93.8833 \\
% \bottomrule
% \end{tabular}
% } 	
\begin{tabular}{cccc}
\toprule
Stats.  & Fixed at a large value    & Balanced exploitation-exploration  
(Ours) & Fixed at a small value  \\
                           
\midrule
\midrule
Avg. Acc. of Top-5 (\%) & 93.262 & \textbf{94.156} & 93.978 \\
Standard Deviation (\%)                             & 0.395 & 0.658 & 0.953  \\ 
\bottomrule
\end{tabular}
} 	

\end{center}
\label{tbl:suppl_guidance_abl}
\vspace{-0.15in}
\end{table}
